# Supplementary material for: Interventional Bag Multi-Instance Learning On Whole-Slide Pathological Images
Source: arXiv:2303.06873 source file (2023-03-13)
Supplement: Supplementary file 1 [file supp_maxmins_c16.tex]

\begin{table}[t]
\caption{Results on Camelyon16 dataset.}
\label{tab:supp_maxmins_C16}
\centering
\resizebox{0.95\linewidth}{!}{
\begin{tabular}{ccccccc}
\toprule
\makecell{Feature \\Extractor}                   & $K$        & Precision   & Recall   & Accuracy   & AUC  \\ \hline
\multirow{5}{*}{ResNet}  & /  & \color{gray}{84.55} &	\color{gray}{75.62} &	\color{gray}{79.84} &	\color{gray}{79.17} \\
                      & 2  & 87.54&	81.39&	84.5&	85.06 \\
                      & 4        & 79.04&	79.37&	79.84&	84.77 \\
                      & 8        & 86.16&	80.74&	83.72&	85.11 \\
                      & 16        & 81.44 &	81.63&	82.17&	84.44 \\
\midrule

\multirow{5}{*}{CTrans}  & /  & \color{gray}{96.39}	& \color{gray}{94.23}	&\color{gray}{95.35} & \color{gray}{95.15} \\
                      & 2        & 96.95&	95.19&	96.12&	95.75 \\
                      & 4        &96.48 &	95.50&	96.12	&95.95 \\
                      & 8        &96.48	 &95.50	&96.12&	95.95 \\
                      & 16        & 96.48 &	95.50&	96.12&	96.00\\

\midrule
\multirow{5}{*}{ViT}  & /  & \color{gray}{93.84}	& \color{gray}{93.24}	&\color{gray}{93.80} & \color{gray}{94.66} \\
                      & 2        & 95.29&	92.31&	93.80&	94.63 \\
                      & 4        &95.29 &	92.31&	93.80&	94.76 \\
                      & 8        &94.21&	92.93&	93.80&	94.66 \\
                      & 16        & 95.29 &	92.31&	93.80&	94.53\\

\bottomrule
\end{tabular}
}
\end{table}
