# Supplementary material for: Interventional Bag Multi-Instance Learning On Whole-Slide Pathological Images
Source: arXiv:2303.06873 source file (2023-03-13)
Supplement: Supplementary file 2 [file supp_maxmins_tcga.tex]

\begin{table}[t]
\caption{Results on TCGA-NSCLC dataset.}
\label{tab:supp_maxmins_tcga}
\centering
\resizebox{0.95\linewidth}{!}{
\begin{tabular}{ccccccc}
\toprule
\makecell{Feature \\Extractor}                   & $K$        & Precision   & Recall   & Accuracy   & AUC  \\ \hline
\multirow{5}{*}{ResNet}  & /  & \color{gray}{88.11}	& \color{gray}{88.12}	&\color{gray}{88.10} & \color{gray}{92.36} \\
                      & 2        & 81.84&	91.86&	79.52&	92.95 \\
                      & 4        &86.13 &	85.71&	85.71&	93.41 \\
                      & 8        &87.49 &	85.78&	85.71&	93.61 \\
                      & 16        & 90.01 &	89.99&	90.00&	94.76\\
\midrule

\multirow{5}{*}{CTrans}  & /  & \color{gray}{94.31}	& \color{gray}{94.27}	&\color{gray}{94.29} & \color{gray}{96.74} \\
                      & 2        & 94.31 &	94.27&	94.29&	97.71 \\
                      & 4        &94.72	& 93.80 &	93.81&	97.71 \\
                      & 8        &94.32 &	94.32&	94.29&	97.80 \\
                      & 16        & 94.31 &	94.27&	94.29&	97.68 \\

\midrule
\multirow{5}{*}{ViT}  & /  & \color{gray}{94.29}	& \color{gray}{94.30}	&\color{gray}{94.29} & \color{gray}{98.15} \\
                      & 2        & 94.77&	94.75&	94.76&	98.17 \\
                      & 4        &93.86	 & 94.77&	93.81&	98.19 \\
                      & 8        &94.77	&94.75&	94.76&	98.22 \\
                      & 16        & 94.77&	94.75&	94.76&	98.26\\

\bottomrule
\end{tabular}
}
\end{table}
